# Supplementary material for: Discovering the Ethereum2 P2P Network
Source: arXiv:2012.14728 source file (2022-09-22)
Supplement: Supplementary file 1 [file appendix.tex]

\section{Appendix}
\subsection{BSC Contribution to the Rumor Repository}

Several months have passed since the BSC-ETH2 got in touch with Rumor. During these months, the team has been able to try and get experienced with the tool while it has been contributing to the development of Rumor by proposing changes or new functionalities, reporting bugs or fixing them.
Summary of the contributions made so far:
\begin{itemize}
    \item Suggested adding a command that allows copying the stdout on the given file. Protolambda added the command $grab$ \cite{grab-commit}.
    \item Reported a bug that was causing a panic runtime error while trying to find the status received from the poll command. @Protolambda fixed the bug \cite{poll-find-received-status-commit}.
    \item Reported a bug that was causing a panic runtime error while trying to poll the status received from the poll command. @Protolambda fixed the bug \cite{poll-received-status-commit}.
    \item Spotted a node deadlock on the scripts/dv5.rumor example. @Protolambda fixed the bug \cite{deadlock-dv5-example}.
    \item Suggested adding a feature to the $dv5 random$ command that automatically adds the founded peers to the peerstore without needing the $next$ command. @Protolambda added the feature with the $-stepwise$ and $--interval$ flags on the $dv5 random$ command \cite{dv5-suggestion}.
    \item Spotted misbehaviour on the libp2p host, it wasn't automatically peering peers from the peerstore following the $--lo-peers$ and $--hi-peers$ flags. Missbehaviour fixed by adding the $peer connectall$ command by @Protolambda \cite{libp2p-host-missbehaviour}.
    \item Spotted a terminal block/freeze while running the command $gossip log$. @Protolambda fixed the bug \cite{gossip-log-freeze}.
    \item Spotted a terminal block/freeze while running the command $gossip events$. @Protolambda fixed the bug \cite{gossip-events-freeze}.
    \item Spotted misbehaviour on the $gossip$ implementation. The $gossip$ command doesn't connect any of the peers on the given $medalla_topic$. Making it unable to log the messages. Spotted the error by the BSC-ETH2 team. The example on the $medalla_gossip.rumor$ had a wrong $fork_digest$ value, it was ussing $0xXXXXXXXX$ while it has to be $XXXXXX$ (without the $0x$ prefix). Pull Request accepted \cite{pull-request-11} fixing the issue on the $medalla_gossip.rumor$ example file.
    % This one is still in progress
    \item Suggestion from @Protolambda to add a shortcut command for each known topic, allowing to parse the fork version in either format. Avoiding the error to happen again.
    \item Spotted misbehaviour on the command $gossip list$, the command just logs 1 topic as much regardless of the real amount of topics joined to. PR suggested by the team fixing the issue \cite{pull-request-13}.
    \item Spotted missing $connectall$ help info when doing $peer --help$. PR suggested by the team fixing the issue \cite{pull-request-13}.
    \item Spotted bug that wouldn't show the peer that sent the gossip message. The team fixed the issue replacing the method used to get the $peer_id$. PR suggested by the team fixing the issue \cite{pull-request-13}.
    \item Spotted panic error while getting the data from a specific peer using the $GetAllData()$ function. Protolambda fixed the bug \cite{get-all-data-bug}. 
\end{itemize}
